# Supplementary material for: Probing the chirality of 1D Majorana edge states around a 2D nanoflake in a superconductor
Source: arXiv:2008.11807 ancillary file (2020-08-26)
Supplement: Supplementary file 1 [file SM.pdf]

# Probing the chirality of 1D Majorana edge states around a 2D nanoflake in a superconductor: Supplemental Material

Andrzej Ptok,[1] David J. Alspaugh,[2] Szczepan Głodzik,[3]
Aksel Kobiałka,[3] Andrzej M. Oleś,[4,5], Pascal Simon[6] and Przemysław Piekarz [1]
[1] *Institute of Nuclear Physics, Polish Academy of Sciences, ul. W. E. Radzikowskiego 152, PL-31342 Kraków, Poland*
[2] *Department of Physics and Astronomy, Louisiana State University, Baton Rouge, Louisiana 70803-4001, USA*
[3] *Institute of Physics, Maria Curie-Skłodowska University, Plac Marii Skłodowskiej-Curie 1, PL-20031 Lublin, Poland*
[4] *Institute of Theoretical Physics, Jagiellonian University, Profesora Stanisława Łojasiewicza 11, PL-30348 Kraków, Poland*
[5] *Max Planck Institute for Solid State Research, Heisenbergstrasse 1, D-70569 Stuttgart, Germany*
[6] *Université Paris-Saclay, CNRS, Laboratoire de Physique des Solides, F-91405, Orsay, France*
(Dated: August 24, 2020)

In this Supplemental Material we present details of analytical calculations (in Sec. S1) as well as additional numerical results in the case of the nanoflake with irregular shape (in Sec. S2).

## S1. DETAILS OF ANALYTICAL CALCULATIONS

### A. Wave function as $r < R_0$

Let us define $H_1(\mathbf{r}, \boldsymbol{\nabla})$ and $H_2(\mathbf{r}, \boldsymbol{\nabla})$ for $r < R_0$ and $r > R_0$, respectively. We have

$$\begin{aligned} H_1(\mathbf{r}, \boldsymbol{\nabla}) &= -\mu_1\sigma_0 + \alpha(\boldsymbol{\sigma} \times -i\boldsymbol{\nabla})_z + h\sigma_z, \\ H_2(\mathbf{r}, \boldsymbol{\nabla}) &= -\mu_2\sigma_0 + \alpha(\boldsymbol{\sigma} \times -i\boldsymbol{\nabla})_z + h\sigma_z. \end{aligned} \tag{S1}$$

Here the system is two-dimensional with $\mathbf{r} = (x, y)$, and the chemical potential is given by

$$\mu(r) = \begin{cases} \mu_1 & r < R_0, \\ \mu_2 & r > R_0. \end{cases} \tag{S2}$$

Let us first focus on $H_1(\mathbf{r}, \boldsymbol{\nabla})$. The second quantized real-space BdG Hamiltonian is given by

$$\mathcal{H}_1 = \frac{1}{2} \int d\mathbf{r}\, \Psi^\dagger(\mathbf{r}) \begin{pmatrix} H_1(\mathbf{r}, \boldsymbol{\nabla}) & i\sigma_y\Delta \\ -i\sigma_y\Delta & -H_1^T(\mathbf{r}, -\boldsymbol{\nabla}) \end{pmatrix} \Psi(\mathbf{r}). \tag{S3}$$

Here $\Psi(\mathbf{r}) = (\psi_\uparrow(\mathbf{r}), \psi_\downarrow(\mathbf{r}), \psi_\uparrow^\dagger(\mathbf{r}), \psi_\downarrow^\dagger(\mathbf{r}))^T$, where $\psi_\sigma(\mathbf{r})$ are electron field operators which destroy an electron at location $\mathbf{r}$. We have that

$$\begin{aligned} \mathcal{H}_1 &= \frac{1}{2} \int d\mathbf{r}\, \Psi^\dagger(\mathbf{r}) \begin{pmatrix} -\mu_1 + h & \alpha e^{-i\theta}(\partial_r - i\frac{1}{r}\partial_\theta) & 0 & \Delta \\ \alpha e^{i\theta}(-\partial_r - i\frac{1}{r}\partial_\theta) & -\mu_1 - h & -\Delta & 0 \\ 0 & -\Delta & \mu_1 - h & \alpha e^{i\theta}(-\partial_r - i\frac{1}{r}\partial_\theta) \\ \Delta & 0 & \alpha e^{-i\theta}(\partial_r - i\frac{1}{r}\partial_\theta) & \mu_1 + h \end{pmatrix} \Psi(\mathbf{r}) \\ &= \frac{1}{2} \int d\mathbf{r} \Psi^\dagger(\mathbf{r}) H_1 \Psi(\mathbf{r}). \end{aligned} \tag{S4}$$

We then wish to find the eigenvectors of $H_1$. That is, we wish to find eigenvectors $\varphi$ such that $H_1\varphi = E\varphi$. Consider the total angular momentum operator,

$$J_z = -i\partial_\theta\tau_0\sigma_0 + \frac{1}{2}\tau_z\sigma_z. \tag{S5}$$

We can verify that this operator commutes with the first quantized Hamiltonian, $[J_z, H_1] = 0$. Thus, the Hamiltonian $H_1$ and the total angular momentum operator $J_z$ have the same eigenstates. The eigenstates of $J_z$ are given by

$$\varphi_n = \begin{pmatrix} u_{n\uparrow}(r)\, e^{i(n-1)\theta} \\ u_{n\downarrow}(r)\, e^{in\theta} \\ v_{n\uparrow}(r)\, e^{in\theta} \\ v_{n\downarrow}(r)\, e^{i(n-1)\theta} \end{pmatrix}. \tag{S6}$$

Here $n$ is an integer, $n \in \mathbb{Z}$, and we may verify that

$$J_z \varphi_n = \left(n - \frac{1}{2}\right)\varphi_n = m_J\, \varphi_n. \tag{S7}$$

Note that the eigenvalues of $J_z$ are half-integer, given by $m_J = n - \frac{1}{2}$. From the expression $H_1\varphi_n = E\varphi_n$ we then obtain the system of equations,

$$\begin{aligned}
(-\mu_1 + h)u_{n\uparrow}(r) + \alpha\left[\partial_r + \frac{n}{r}\right]u_{n\downarrow}(r) + \Delta v_{n\downarrow}(r) &= Eu_{n\uparrow}(r),\\
\alpha\left[-\partial_r + \frac{n-1}{r}\right]u_{n\uparrow}(r) + (-\mu_1 - h)u_{n\downarrow}(r) - \Delta v_{n\uparrow}(r) &= Eu_{n\downarrow}(r),\\
-\Delta u_{n\downarrow}(r) + (\mu_1 - h)v_{n\uparrow}(r) + \alpha\left[-\partial_r + \frac{n-1}{r}\right]v_{n\downarrow}(r) &= Ev_{n\uparrow}(r),\\
\Delta u_{n\uparrow}(r) + \alpha\left[\partial_r + \frac{n}{r}\right]v_{n\uparrow}(r) + (\mu_1 + h)v_{n\downarrow}(r) &= Ev_{n\downarrow}(r).
\end{aligned} \tag{S8}$$

Now, we expect to find a localized state at $r = R_0$, which decays as $r \to 0$ and $r \to \infty$. That is, for the $r < R_0$ region, we expect the $\{u\}$ and $\{v\}$ functions to be related to the Modified Bessel Functions of the First Kind $I_n(kr)$, which are finite as $r = 0$. Here, $k$ is the radial momentum. The Modified Bessel Functions of the First Kind obey the following recurrence relations:

$$\frac{n}{kr}I_n(kr) = \frac{1}{2}\Big(I_{n-1}(kr) - I_{n+1}(kr)\Big), \tag{S9}$$

$$\partial_{kr}I_n(kr) = \frac{1}{2}\Big(I_{n-1}(kr) + I_{n+1}(kr)\Big). \tag{S10}$$

From these, we may find that

$$\begin{aligned}
\left[\partial_r + \frac{n}{r}\right]I_n(kr) &= kI_{n-1}(kr),\\
\left[-\partial_r + \frac{n-1}{r}\right]I_{n-1}(kr) &= -kI_n(kr).
\end{aligned} \tag{S11}$$

Let us then assume that our vector has the form

$$\varphi_n = \begin{pmatrix} aI_{n-1}(kr)\, e^{i(n-1)\theta} \\ bI_n(kr)\, e^{in\theta} \\ cI_n(kr)\, e^{in\theta} \\ dI_{n-1}(kr)\, e^{i(n-1)\theta} \end{pmatrix}. \tag{S12}$$

With this assumption, our system of equations then has the form

$$\begin{aligned}
(-\mu_1 + h)a + \alpha kb + \Delta d &= Ea,\\
-\alpha ka + (-\mu_1 - h)b - \Delta c &= Eb,\\
-\Delta b + (\mu_1 - h)c - \alpha kd &= Ec,\\
\Delta a + \alpha kc + (\mu_1 + h)d &= Ed.
\end{aligned} \tag{S13}$$

$$\begin{pmatrix} -\mu_1 + h - E & \alpha k & 0 & \Delta \\ -\alpha k & -\mu_1 - h - E & -\Delta & 0 \\ 0 & -\Delta & \mu_1 - h - E & -\alpha k \\ \Delta & 0 & \alpha k & \mu_1 + h - E \end{pmatrix}\begin{pmatrix} a \\ b \\ c \\ d \end{pmatrix} = \begin{pmatrix} 0 \\ 0 \\ 0 \\ 0 \end{pmatrix}. \tag{S14}$$

Setting the determinant to zero gives

$$k_\pm = \frac{1}{\alpha}\sqrt{h^2 - E^2 + \Delta^2 - \mu_1^2 \pm 2\sqrt{E^2\mu_1^2 + \Delta^2(h - \mu_1)(h + \mu_1)}}, \tag{S15}$$

and

$$a_\pm = \frac{-E\mu_1 \pm \sqrt{h^2\Delta^2 + (E-\Delta)(E+\Delta)\mu_1^2}}{\Delta(h-\mu_1)}, \tag{S16}$$

$$b_\pm = \frac{(E\mu_1 \mp \sqrt{h^2\Delta^2 + (E-\Delta)(E+\Delta)\mu_1^2})(\sqrt{h^2 - E^2 + \Delta^2 - \mu_1^2 \pm 2\sqrt{E^2\mu_1^2 + \Delta^2(h-\mu_1)(h+\mu_1)}})}{\Delta[h(h+E) - \mu_1^2 \pm \sqrt{h^2\Delta^2 + (E-\Delta)(E+\Delta)\mu_1^2}]}, \tag{S17}$$

$$c_\pm = -\frac{(h+\mu_1)\sqrt{h^2 - E^2 + \Delta^2 - \mu_1^2 \pm 2\sqrt{E^2\mu_1^2 + \Delta^2(h-\mu_1)(h+\mu_1)}}}{h(h+E) - \mu_1^2 \pm \sqrt{h^2\Delta^2 + (E-\Delta)(E+\Delta)\mu_1^2}}, \tag{S18}$$

$$d_\pm = 1. \tag{S19}$$

The wave function as $r < R_0$ then has the generic form,

$$\varphi_n(r) = N_n^+ \begin{pmatrix} a_+ I_{n-1}(k_+ r)e^{i(n-1)\theta} \\ b_+ I_n(k_+ r)e^{in\theta} \\ c_+ I_n(k_+ r)e^{in\theta} \\ I_{n-1}(k_+ r)e^{i(n-1)\theta} \end{pmatrix} + N_n^- \begin{pmatrix} a_- I_{n-1}(k_- r)e^{i(n-1)\theta} \\ b_- I_n(k_- r)e^{in\theta} \\ c_- I_n(k_- r)e^{in\theta} \\ I_{n-1}(k_- r)e^{i(n-1)\theta} \end{pmatrix}. \tag{S20}$$

Here $N_n^\pm$ are normalization constants.

### B. Wave function as $r > R_0$

We can then repeat this analysis for the region $r > R_0$. The analysis will then be the same, except that the chemical potential will be given by $\mu_2$. In the $r > R_0$ region, the wave function must decay as $r \to \infty$. Thus, we must use the Modified Bessel Functions of the Second Kind $K_n(kr)$. However, these objects do not satisfy the same recurrence relations. Instead, the object $e^{in\pi}K_n(kr)$ satisfies the following recurrence relations:

$$\frac{n}{kr}[e^{in\pi}K_n(kr)] = \frac{1}{2}\Big(e^{i(n-1)\pi}K_{n-1}(kr) - e^{i(n+1)\pi}K_{n+1}(kr)\Big), \tag{S21}$$

$$\partial_{kr}[e^{in\pi}K_n(kr)] = \frac{1}{2}\Big(e^{i(n-1)\pi}K_{n-1}(kr) + e^{i(n+1)\pi}K_{n+1}(kr)\Big).$$

From these, we may find that

$$\Big[\partial_r + \frac{n}{r}\Big]e^{in\pi}K_n(kr) = ke^{i(n-1)\pi}K_{n-1}(kr), \tag{S22}$$

$$\Big[-\partial_r + \frac{n-1}{r}\Big]e^{i(n-1)\pi}K_{n-1}(kr) = -ke^{in\pi}K_n(kr). \tag{S23}$$

Following similar steps as in the previous section, we may find that the wave function then has the form,

$$\widetilde{\varphi}_n(r) = \widetilde{N}_n^+ \begin{pmatrix} \widetilde{a}_+ e^{i(n-1)\pi}K_{n-1}(\widetilde{k}_+ r)e^{i(n-1)\theta} \\ \widetilde{b}_+ e^{in\pi}K_n(\widetilde{k}_+ r)e^{in\theta} \\ \widetilde{c}_+ e^{in\pi}K_n(\widetilde{k}_+ r)e^{in\theta} \\ e^{i(n-1)\pi}K_{n-1}(\widetilde{k}_+ r)e^{i(n-1)\theta} \end{pmatrix} + \widetilde{N}_n^- \begin{pmatrix} \widetilde{a}_- e^{i(n-1)\pi}K_{n-1}(\widetilde{k}_- r)e^{i(n-1)\theta} \\ \widetilde{b}_- e^{in\pi}K_n(\widetilde{k}_- r)e^{in\theta} \\ \widetilde{c}_- e^{in\pi}K_n(\widetilde{k}_- r)e^{in\theta} \\ e^{i(n-1)\pi}K_{n-1}(\widetilde{k}_- r)e^{i(n-1)\theta} \end{pmatrix}. \tag{S24}$$

Here the parameters $\{\widetilde{k}_\pm, \widetilde{a}_\pm, \widetilde{b}_\pm, \widetilde{c}_\pm\}$ have the same form as those given in the previous section, except that we replace $\mu_1 \to \mu_2$.

### C. Expression for the bound state energy

Matching the wave functions at $r = R_0$, we obtain $\varphi_n(R_0) = \widetilde{\varphi}_n(R_0)$. This expression gives us the system of equations,

$$\begin{aligned}
N_n^+ a_+ I_{n-1}(k_+R_0) + N_n^- a_- I_{n-1}(k_-R_0) &= \widetilde{N}_n^+ \widetilde{a}_+ e^{i(n-1)\pi} K_{n-1}(\widetilde{k}_+R_0) + \widetilde{N}_n^- \widetilde{a}_- e^{i(n-1)\pi} K_{n-1}(\widetilde{k}_-R_0),\\
N_n^+ b_+ I_n(k_+R_0) + N_n^- b_- I_n(k_-R_0) &= \widetilde{N}_n^+ \widetilde{b}_+ e^{in\pi} K_n(\widetilde{k}_+R_0) + \widetilde{N}_n^- \widetilde{b}_- e^{in\pi} K_n(\widetilde{k}_-R_0),\\
N_n^+ c_+ I_n(k_+R_0) + N_n^- c_- I_n(k_-R_0) &= \widetilde{N}_n^+ \widetilde{c}_+ e^{in\pi} K_n(\widetilde{k}_+R_0) + \widetilde{N}_n^- \widetilde{c}_- e^{in\pi} K_n(\widetilde{k}_-R_0),\\
N_n^+ I_{n-1}(k_+R_0) + N_n^- I_{n-1}(k_-R_0) &= \widetilde{N}_n^+ e^{i(n-1)\pi} K_{n-1}(\widetilde{k}_+R_0) + \widetilde{N}_n^- e^{i(n-1)\pi} K_{n-1}(\widetilde{k}_-R_0).
\end{aligned} \tag{S25}$$

Rewriting these gives,

$$\begin{pmatrix} a_+ I_{n-1}(k_+R_0) & a_- I_{n-1}(k_-R_0) & -\widetilde{a}_+ e^{i(n-1)\pi} K_{n-1}(\widetilde{k}_+R_0) & -\widetilde{a}_- e^{i(n-1)\pi} K_{n-1}(\widetilde{k}_-R_0) \\ b_+ I_n(k_+R_0) & b_- I_n(k_-R_0) & -\widetilde{b}_+ e^{in\pi} K_n(\widetilde{k}_+R_0) & -\widetilde{b}_- e^{in\pi} K_n(\widetilde{k}_-R_0) \\ c_+ I_n(k_+R_0) & c_- I_n(k_-R_0) & -\widetilde{c}_+ e^{in\pi} K_n(\widetilde{k}_+R_0) & -\widetilde{c}_- e^{in\pi} K_n(\widetilde{k}_-R_0) \\ I_{n-1}(k_+R_0) & I_{n-1}(k_-R_0) & -e^{i(n-1)\pi} K_{n-1}(\widetilde{k}_+R_0) & -e^{i(n-1)\pi} K_{n-1}(\widetilde{k}_-R_0) \end{pmatrix} \begin{pmatrix} N_n^+ \\ N_n^- \\ \widetilde{N}_n^+ \\ \widetilde{N}_n^- \end{pmatrix} = \begin{pmatrix} 0 \\ 0 \\ 0 \\ 0 \end{pmatrix}. \tag{S26}$$

In order to have a nontrivial bound state, the determinant of the above matrix must be equal to zero. Finding the determinant and setting it to zero, we then obtain the expression,

$$\begin{aligned}
& I_n(k_-R_0)\Big\{ -(\widetilde{a}_- - \widetilde{a}_+)(b_+c_- - b_-c_+) I_n(k_+R_0) K_{n-1}(\widetilde{k}_-R_0) K_{n-1}(\widetilde{k}_+R_0) \\
&\quad + I_{n-1}(k_+R_0)\Big[(-a_+ + \widetilde{a}_+)(\widetilde{b}_-c_- - b_-\widetilde{c}_-) K_{n-1}(\widetilde{k}_+R_0) K_n(\widetilde{k}_-R_0) \\
&\quad + (\widetilde{a}_- + a_+)(\widetilde{b}_+c_- - b_-\widetilde{c}_+) K_{n-1}(\widetilde{k}_-R_0) K_n(\widetilde{k}_+R_0)\Big]\Big\} \\
& + I_{n-1}(k_-R_0)\Big\{(-a_- + a_+)(\widetilde{b}_+\widetilde{c}_- - \widetilde{b}_-\widetilde{c}_+) I_{n-1}(k_+R_0) K_n(\widetilde{k}_-R_0) K_n(\widetilde{k}_+R_0) \\
&\quad + I_n(k_+R_0)\Big[(-a_- + \widetilde{a}_+)(b_+\widetilde{c}_- - \widetilde{b}_-c_+) K_{n-1}(\widetilde{k}_+R_0) K_n(\widetilde{k}_-R_0) \\
&\quad + (-a_- + \widetilde{a}_-)(\widetilde{b}_+c_+ - b_+\widetilde{c}_+) K_{n-1}(\widetilde{k}_-R_0) K_n(\widetilde{k}_+R_0)\Big]\Big\} = 0.
\end{aligned} \tag{S27}$$

This is then a transcendental equation which must be numerically solved for the energy $E$.

## S2. NANOFLAKE WITH IRREGULAR SHAPE

In this Supplemental Material we present additional results for different parameters of a nanoflake. We present here results for nanoflake with irregular shape (Fig. S1), and parameters similar like in main text: $\lambda = 1$, $V_0/t = -0.06$. In some figures we compare impact of the smearing of the domain wall into results [i.e. at Fig. S2, S3, and S4, panels from (a) to (c) correspond to pairs of parameters $(\lambda, V_0/t) = (0.25, -0.25)$, $(1.0, -0.06)$, and $(4.0, -0.005)$, respectively].

- Fig. S1 - presents shape of the nanoflake with irregular shape,
- Fig. S2 - presents impact of the domain wall smearing into indicator $\chi$ — smearing of the domain wall given by the $\lambda$ (length of decay of the impurity potential) leads to modification of the domain wall width; additionally, in the case of the sharp smearing (panel a), we can observe bigger impact of the disorder into the topological phase inside nanoflake (i.e. by green arrow we show places where locally the topological phase is not induced by the nanoflake potential),
- Fig. S3 - presents an impact of the domain wall smearing into bond current — in this example we show how the smearing of the domain wall influences the bond current localization as it becomes more space-extensive; increasing of the domain wall smearing leads to decrease in the value of the bond current.

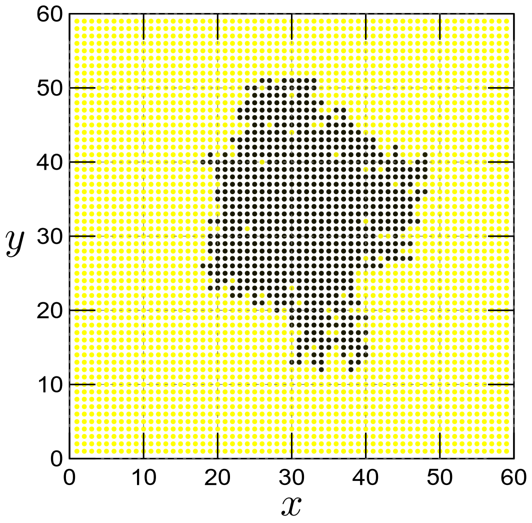


FIG. S1. Rendered shape of the nanoflake used in the calculations. Black circles (yellow circles) correspond to the substituted (substrate) atoms. Underlying square lattice dimensions: $N_x \times N_y = 59 \times 59$. Approximately 20% of the lattice is covered by nanoflake.

- Fig. S4 - localization of the in-gap state dependent on smearing of the domain wall — effect similar to observed above, in the case of the LDOS of the in-gap states; increase of the domain wall smearing leads to decrease of the spectral weight,
- Fig. S5 - LDOS along nanoflake — crossection of the LDOS along the nanoflake in practice has the same form like in the case of the circular nanoflake (cf. main text),
- Fig. S6 and Fig. S7 - partial DOS for bulk states, nanoflake states and domain wall — here, we compare the partial DOS depending on how we define *domain wall* (cf. main text); independent of definition, the in-gap states are observed in the same form for $h$ in range given by topological phase transition in the case of the circular nanoflake.
- Fig. S8 - partial DOS for few values of the magnetic field — here, we show how magnetic field changes partial DOS (shift of the spectral weight from the domain wall in-gap states to bulk states),
- Fig. S9 - spectrum of the system in function of magnetic field and below, a corresponding change in the value of $\chi$ — this example shows exact dependence between $\chi$ and topological phases; in the case of the homogeneous system (green and red dots), the topological phase transition occurs in $h_{c2}$ and $h_c$. Emergence of non–trivial phase in nanoflake leads to occurrence of in-gap states in range $h_{c2} < h < h_c$.
- Fig. S10 - topological phase diagram — the form the topological phase diagram is in practice independent on the shape of the nanoflake and has the same form as in the case of the circular nanoflake (cf. main text).

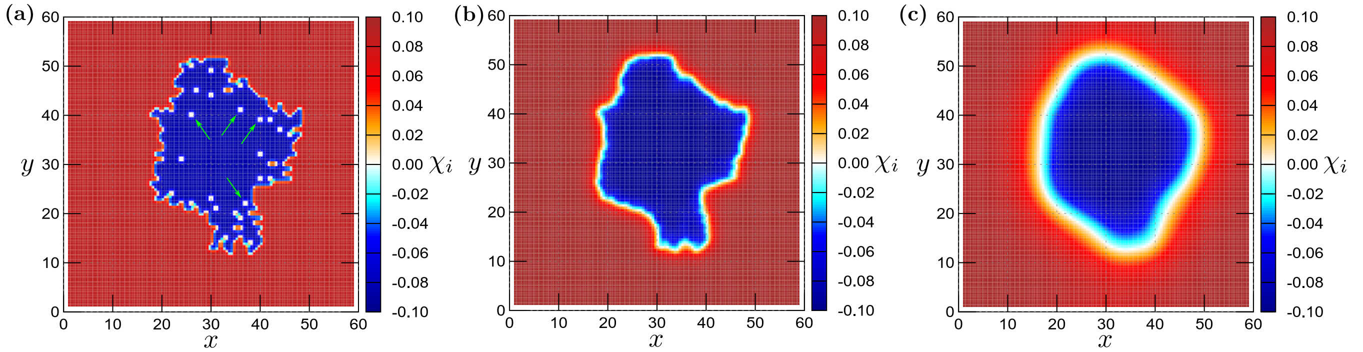


FIG. S2. Real space map of the indicator $\chi_i$ [cf. Eq. (22) in the main text] describing existence of the non–trivial topological phase (blue color denotes negative value of $\chi_i$).

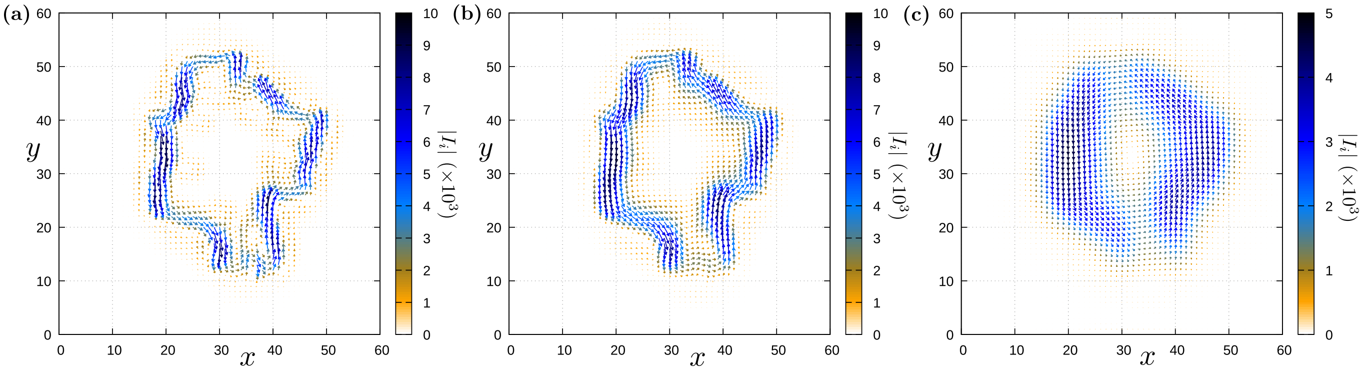


FIG. S3. Bond currents — color corresponds to the absolute value of the current $|I_i|$.

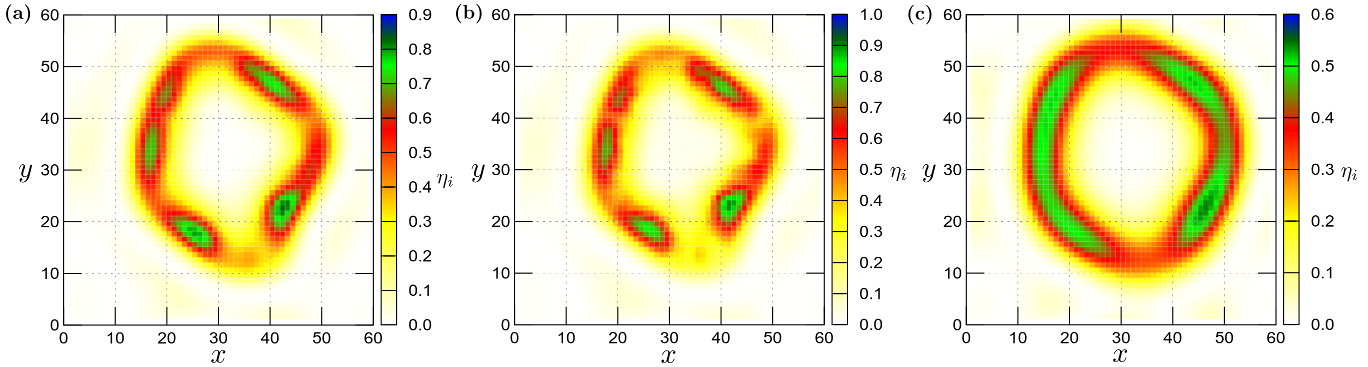


FIG. S4. The localization of the first eigenstate below Fermi level.

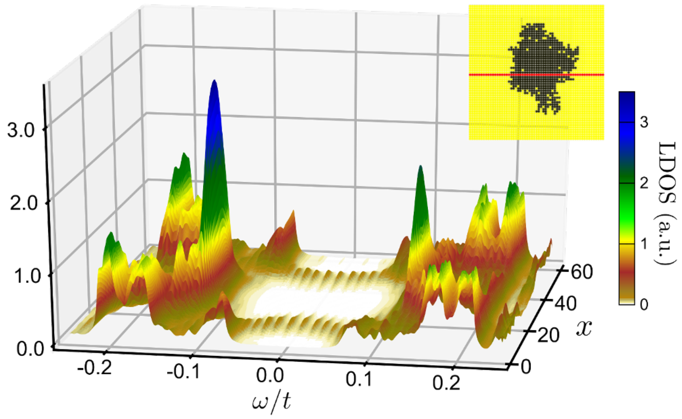


FIG. S5. Local density of states along the line presented in the inset.

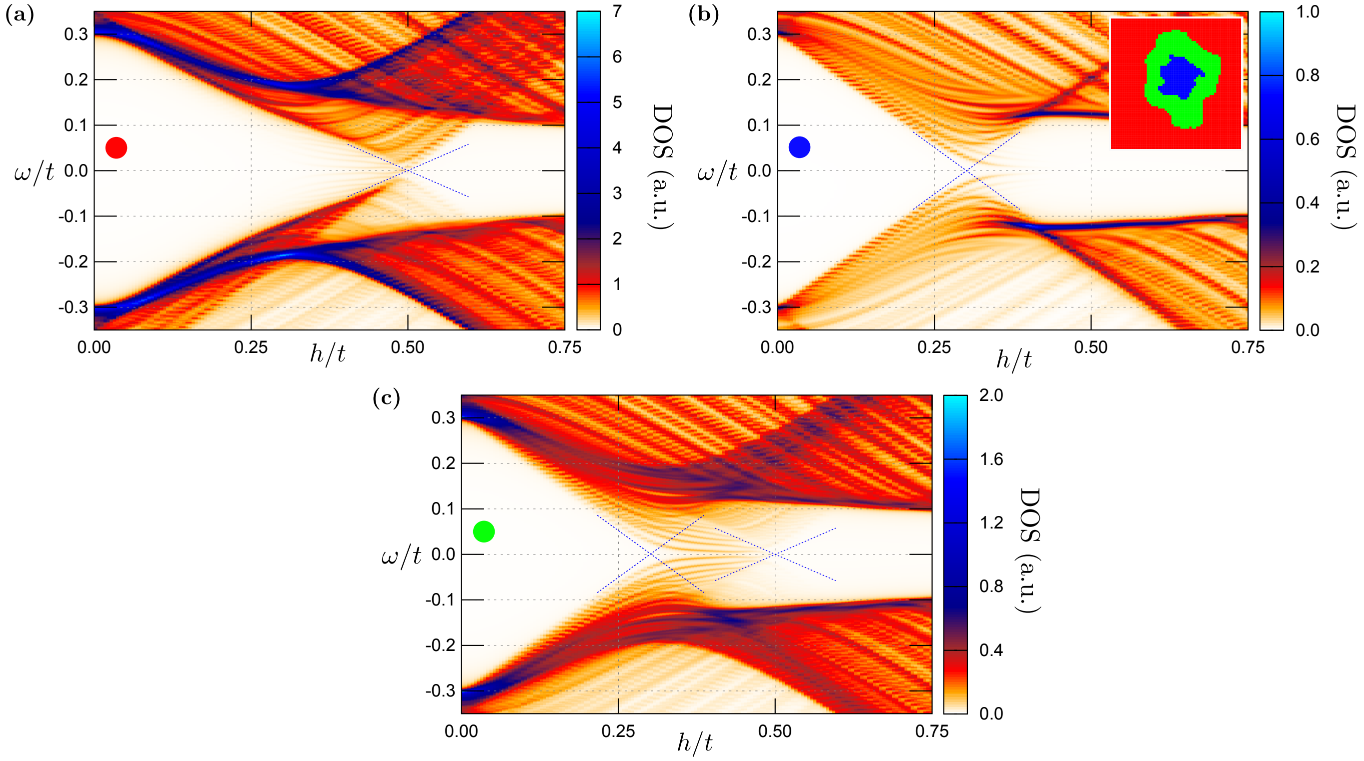


FIG. S6. Partial density of states for different regions: (a) bulk, (b) nanoflake, and (c) domain wall. Blue dashed lines serve as a guide to the eye and present the linear continuation of the gap closing. Results similar to Fig. S6 but for different conditions defining regions of system: nanoflake for $|V_i| < 0.95 \max |V_i|$, bulk for $|V_i| > 0.05 \max |V_i|$, and domain wall otherwise.

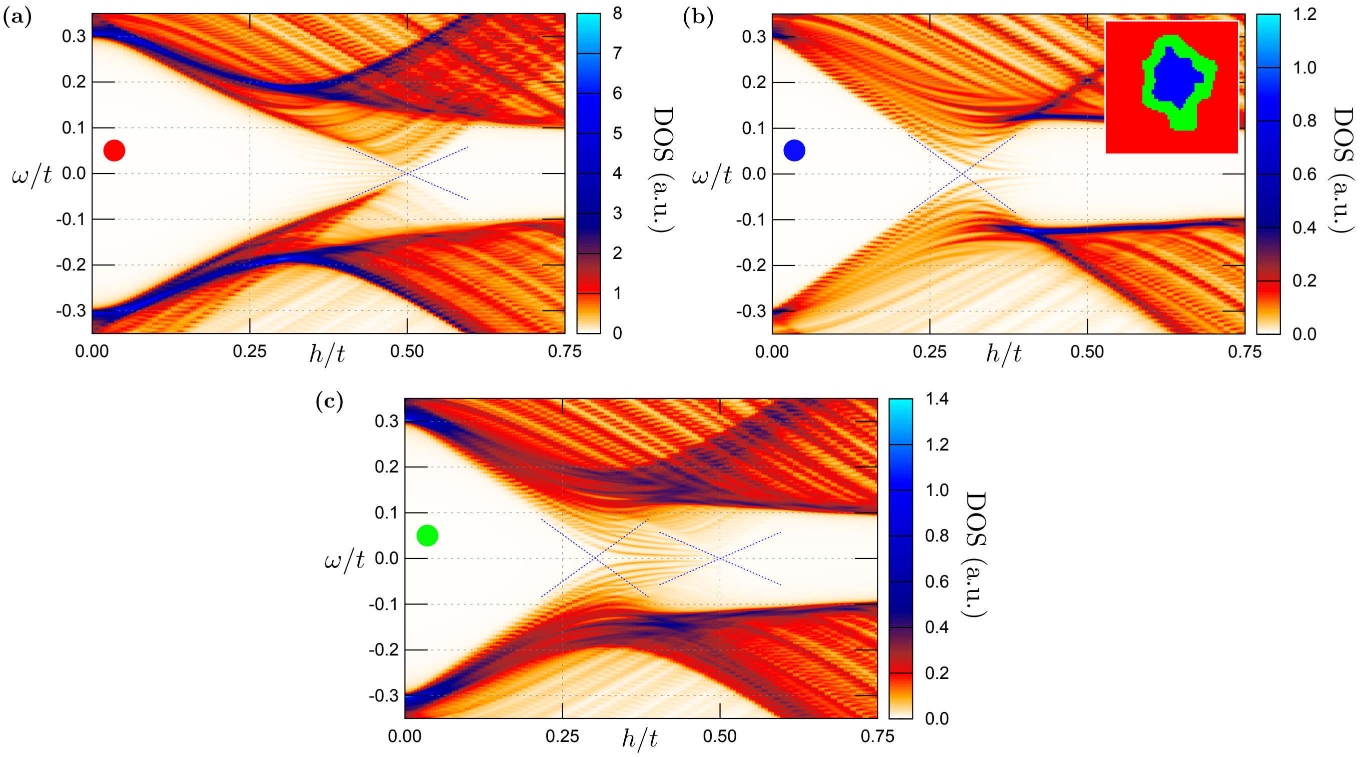


FIG. S7. Partial density of states for different regions: (a) bulk, (b) nanoflake, and (c) domain wall. Blue dashed lines serve as a guide to the eye and present the linear continuation of the gap closing. Results similar to Fig. S6 but for different conditions defining regions of system: nanoflake for $|V_i| < 0.90 \max |V_i|$, bulk for $|V_i| > 0.10 \max |V_i|$, and domain wall otherwise.

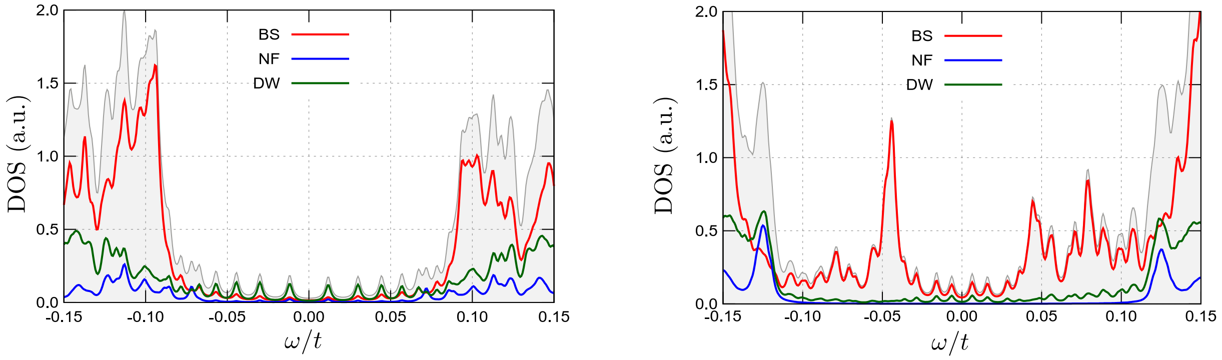


FIG. S8. Partial density of states for the nanoflake with parameters the same as in Fig. S2(b). Red, blue and green line correspond to the bulk system (BS — red line), nanoflake (NF — blue line), and domain wall (DW — green line) contribution to the total density of states (marked by gray color), respectively. Results for an effective magnetic field $h$ equal $0.35t$ (left) and $0.45t$ (right).

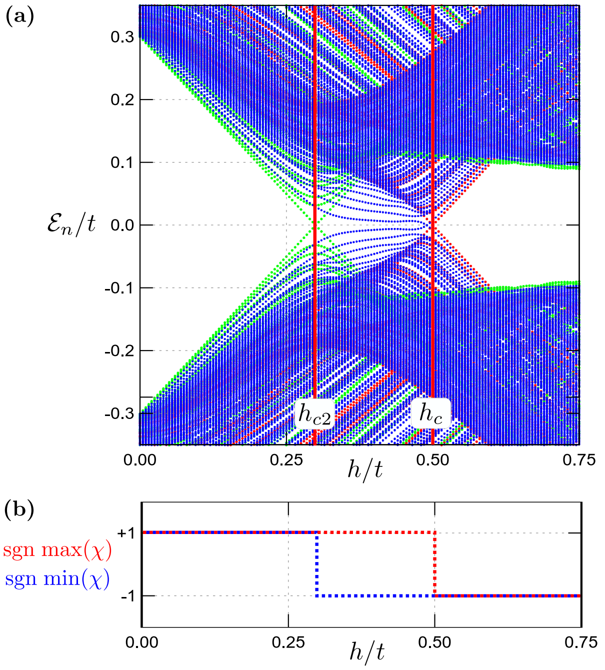


FIG. S9. Analysis of the spectrum of the system as a function of the magnetic field $h/t$, with: (a) gap closing and level crossing (green states) and (b) changes in the sign of minimal (blue) and maximal (red) value of $\chi_i$ indicator.

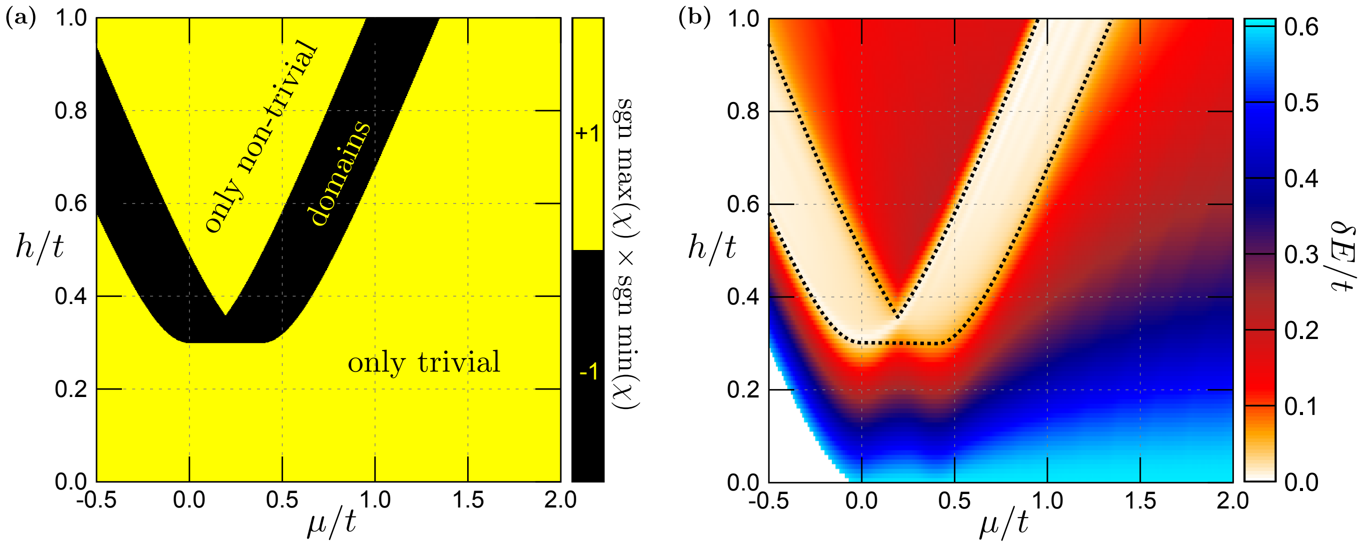


FIG. S10. Topological phase diagram— in the $(\mu, h)$ plane: (a) as obtained from indicator $\chi_i$ and (b) the value of the energy gap $\delta E$. Note that the values in bottom left corner are very high and exceed the scale of the plot.
